# Supplementary material for: How do Quadratic Regularizers Prevent Catastrophic Forgetting: The Role of Interpolation
Source: arXiv:2102.02805 source file (2022-08-12)
Supplement: Supplementary file 1 [file prox.tex]

\section{EMR as Proximal Gradient Descent}
\label{sec:prox}
We now demonstrate EMR is equivalent to using \emph{proximal} gradient descent to solve an adaptive quadratic regularization problem. Specifically, we see the weighted averaging step in EMR is in fact a proximal operation.

Define a function $f(x) = \norm{\sqrt{\frac{R_{j}}{1-R_{j}}} \odot \left(x - \theta_{n-1}^{*}\right)}^{2}$. We note $f(x)$ has the following proximal operator:
\begin{equation}
\label{eq:proxop}
\begin{split}
\text{prox}_{f}(v) &= \argmin_{x} \frac{1}{2} \norm{\sqrt{\frac{R_{j}}{1-R_{j}}} \odot \left(x - \theta_{n-1}^{*}\right)}^{2} + \frac{1}{2} \norm{x - v}^{2}\\
				   &= \left(1 - R_{j}\right) \odot v + R_{j} \odot \theta_{n-1}^{*}
\end{split}
\end{equation}

Now consider the following quadratic regularization loss for learning the $n^{\text{th}}$ task:
\begin{equation}
\label{eq:proxloss}
L = L_{T_{n}} + \frac{1}{2} \norm{\sqrt{\frac{R_{j}}{1-R_{j}}} \odot \left(\theta_{n} - \theta_{n-1}^{*}\right)}^{2}.
\end{equation}

The regularization loss in \autoref{eq:proxloss} has a closed-form proximal operator (see \autoref{eq:proxop}). Therefore, we can employ proximal gradient descent to solve this problem, resulting in the following updates:
\begin{equation} 
\begin{split}
\text{(i)}\, \theta_{n} &\to \theta_{n} - \eta \nabla_{\theta_{n}} L_{T_{n}} \quad\quad\, \text{{\small (Gradient descent) ;}}\\
\text{(ii)}\, \theta_{n} &\to \text{prox}_{f}(\theta_{n}) = \left(1-R_{j}\right) \odot \theta_{n} + R_{j} \odot \theta_{n-1}^{*} \quad \text{{\small (Prox.\ operation)}}.\\
\end{split}
\end{equation}

These steps are exactly equal to the operations involved in EMR (see Equation~8 from main paper). This shows the weighted averaging operation in EMR is in fact the proximal operation for $f(x) = \norm{\sqrt{\frac{R_{j}}{1-R_{j}}} \odot \left(x - \theta_{n-1}^{*}\right)}^{2}$ and, overall, EMR is solving the following quadratic regularization problem:
\begin{equation}
L = L_{T_{n}} + \frac{1}{2} \norm{\sqrt{\frac{R_{j}}{1-R_{j}}} \odot \left(\theta_{n} - \theta_{n-1}^{*}\right)}^{2}.
\end{equation}

Further, when the relative importance measure used in EMR is substituted (Equation~10 from main paper) in the above equation, the $j^{\text{th}}$ EMR iteration is equivalent to using proximal gradient descent to solve the following quadratic regularization problem:
\begin{equation}
\label{eq:proxloss_repeat}
L = L_{T_{n}} + \frac{1}{2} \norm{\left(\left|\frac{\alpha_{n-1}}{\alpha_{T_{n}}}\right|\right)^{1/4} \odot \left(\theta_{n} - \theta_{n-1}^{*}\right)}^{2}.
\end{equation}
Therefore, we see \emph{EMR solves a quadratic regularization problem whose regularization loss adapts each iteration based upon the relative importance of a parameter for previous tasks versus current task.}
